# Supplementary material for: VQ3D: Learning a 3D-Aware Generative Model on ImageNet
Source: arXiv:2302.06833 source file (2023-02-14)
Supplement: Supplementary file 1 [file appendix.tex]

\todo{List things that did not work}
